# Supplementary material for: Transferring an analysis of human brain organization to language models
Source: arXiv:2611.24626 source file (2026-11-18)
Supplement: Supplementary file 2 [file olmo_correct_rows.tex]

0--6 & 30.0 & 31.3 & 28.0 & 27.3 & 23.0 & 23.7 & 22.7 & 22.3 \\
2--8 & 30.7 & 32.0 & 29.0 & 31.0 & 30.7 & 30.7 & 29.3 & 30.3 \\
4--10 & 33.0 & 34.3 & 33.7 & 35.3 & 32.3 & 35.0 & 30.0 & 36.7 \\
6--12 & 38.3 & 40.7 & 39.3 & 42.7 & 46.3 & 42.7 & 40.0 & 39.0 \\
8--14 & 35.0 & 41.0 & 37.7 & 41.3 & 44.7 & 47.3 & 40.7 & 41.7 \\
10--16 & 40.0 & 34.3 & 40.7 & 39.3 & 37.7 & 39.3 & 37.3 & 37.3 \\
12--18 & 38.3 & 35.7 & 39.3 & 41.3 & 41.7 & 42.7 & 40.7 & 42.7 \\
14--20 & 39.0 & 37.7 & 38.7 & 38.7 & 36.0 & 38.3 & 40.3 & 43.0 \\
16--22 & 34.7 & 39.7 & 39.0 & 38.0 & 41.3 & 37.3 & 39.0 & 37.7 \\
18--24 & 36.3 & 35.7 & 42.0 & 39.0 & 39.0 & 39.3 & 39.7 & 40.0 \\
20--26 & 34.0 & 35.3 & 40.0 & 41.7 & 34.0 & 36.0 & 36.3 & 40.3 \\
22--28 & 35.0 & 38.0 & 36.3 & 39.7 & 40.0 & 39.7 & 40.0 & 44.7 \\
24--30 & 36.7 & 40.0 & 42.0 & 42.3 & 33.3 & 25.7 & 14.0 & 12.3 \\
