# Supplementary material for: Transferring an analysis of human brain organization to language models
Source: arXiv:2611.24626 source file (2026-11-18)
Supplement: Supplementary file 3 [file olmo_endpoint_rows.tex]

0--6 & 26/19/22 & $-$14.2 & 38.4 & 16.7 & 15/4/8 & 19/24/21 \\
2--8 & 37/28/26 & $-$5.0 & 50.8 & 23.5 & 22/7/9 & 15/18/18 \\
4--10 & 38/37/35 & +2.3 & 60.6 & 29.7 & 19/12/16 & 11/14/16 \\
6--12 & 44/39/34 & +5.0 & 65.2 & 30.6 & 24/11/14 & 10/11/15 \\
8--14 & 45/38/42 & +8.0 & 72.0 & 32.3 & 20/13/18 & 5/14/11 \\
10--16 & 36/37/39 & +3.1 & 65.8 & 28.1 & 15/13/16 & 9/15/12 \\
12--18 & 41/43/44 & +9.2 & 74.2 & 32.4 & 18/14/19 & 7/10/10 \\
14--20 & 41/43/45 & +9.6 & 71.5 & 34.1 & 22/13/19 & 11/9/9 \\
16--22 & 41/35/37 & +3.4 & 61.6 & 30.8 & 22/11/16 & 11/15/14 \\
18--24 & 45/36/39 & +6.1 & 67.1 & 32.1 & 22/13/16 & 7/16/12 \\
20--26 & 46/36/39 & +6.5 & 65.9 & 33.3 & 24/12/17 & 8/15/13 \\
22--28 & 51/41/42 & +11.5 & 75.9 & 35.3 & 24/14/18 & 3/12/11 \\
24--30 & 12/11/14 & $-$25.7 & 23.2 & 8.2 & 5/3/5 & 23/31/26 \\
