# Supplementary material for: Transferring an analysis of human brain organization to language models
Source: arXiv:2611.24626 source file (2026-11-18)
Supplement: Supplementary file 4 [file policy_R_rows.tex]

M3B & MATH-87 & 85 & $-$0.077 & 0.085 & 0.218 & 0.142 \\
M3B & AIME 2024 & 30 & $-$0.030 & 0.143 & 0.231 & 0.134 \\
M3B & AIME 2025 & 30 & $-$0.074 & 0.117 & 0.243 & 0.150 \\
Q7B & MATH-87 & 80 & 0.428 & 0.629 & 0.684 & 0.699 \\
Q7B & AIME 2024 & 30 & 0.428 & 0.634 & 0.697 & 0.711 \\
Q7B & AIME 2025 & 30 & 0.435 & 0.627 & 0.691 & 0.705 \\
M8B & MATH-87 & 87 & $-$0.179 & $-$0.518 & $-$0.556 & $-$0.386 \\
M8B & AIME 2024 & 30 & $-$0.151 & $-$0.403 & $-$0.474 & $-$0.319 \\
M8B & AIME 2025 & 30 & $-$0.141 & $-$0.484 & $-$0.530 & $-$0.384 \\
L8B & MATH-87 & 76 & 0.086 & 0.244 & 0.273 & 0.270 \\
L8B & AIME 2024 & 30 & 0.079 & 0.223 & 0.253 & 0.243 \\
L8B & AIME 2025 & 30 & 0.077 & 0.223 & 0.253 & 0.247 \\
Q14B & MATH-87 & 82 & 0.076 & 0.288 & 0.339 & 0.353 \\
Q14B & AIME 2024 & 30 & 0.055 & 0.278 & 0.339 & 0.352 \\
Q14B & AIME 2025 & 30 & 0.059 & 0.278 & 0.336 & 0.350 \\
M14B & MATH-87 & 85 & $-$0.254 & $-$0.191 & $-$0.173 & $-$0.163 \\
M14B & AIME 2024 & 30 & $-$0.248 & $-$0.139 & $-$0.145 & $-$0.151 \\
M14B & AIME 2025 & 30 & $-$0.268 & $-$0.155 & $-$0.145 & $-$0.153 \\
