# Supplementary material for: Transferring an analysis of human brain organization to language models
Source: arXiv:2611.24626 source file (2026-11-18)
Supplement: Supplementary file 5 [file policy_count_rows.tex]

M3B & 6 & 2 & 2 & 1 & 11 \\
Q7B & 5 & 4 & 2 & 1 & 12 \\
M8B & 10 & 2 & 2 & 1 & 15 \\
L8B & 6 & 2 & 4 & 1 & 13 \\
Q14B & 15 & 4 & 2 & 1 & 22 \\
M14B & 16 & 2 & 2 & 1 & 21 \\
