# Supplementary material for: Transferring an analysis of human brain organization to language models
Source: arXiv:2611.24626 source file (2026-11-18)
Supplement: Supplementary file 6 [file policy_pos_rows_no_n.tex]

M3B & MATH-87 & 0.391 & 0.572 & 0.671 & 0.654 \\
M3B & AIME 2024 & 0.348 & 0.524 & 0.627 & 0.604 \\
M3B & AIME 2025 & 0.309 & 0.516 & 0.624 & 0.580 \\
Q7B & MATH-87 & 0.142 & 0.230 & 0.348 & 0.320 \\
Q7B & AIME 2024 & 0.162 & 0.375 & 0.624 & 0.680 \\
Q7B & AIME 2025 & 0.095 & 0.180 & 0.425 & 0.524 \\
M8B & MATH-87 & 0.388 & 0.370 & 0.156 & 0.173 \\
M8B & AIME 2024 & 0.381 & 0.327 & 0.141 & 0.081 \\
M8B & AIME 2025 & 0.388 & 0.332 & 0.177 & 0.063 \\
L8B & MATH-87 & $-$0.149 & 0.109 & 0.128 & 0.089 \\
L8B & AIME 2024 & $-$0.072 & 0.148 & 0.134 & 0.139 \\
L8B & AIME 2025 & $-$0.041 & 0.161 & 0.160 & 0.168 \\
Q14B & MATH-87 & $-$0.033 & 0.199 & 0.243 & 0.258 \\
Q14B & AIME 2024 & $-$0.014 & 0.180 & 0.259 & 0.277 \\
Q14B & AIME 2025 & 0.052 & 0.253 & 0.344 & 0.384 \\
M14B & MATH-87 & 0.082 & 0.247 & 0.262 & 0.293 \\
M14B & AIME 2024 & 0.076 & 0.250 & 0.287 & 0.302 \\
M14B & AIME 2025 & 0.056 & 0.244 & 0.293 & 0.322 \\
