# Supplementary material for: Transferring an analysis of human brain organization to language models
Source: arXiv:2611.24626 source file (2026-11-18)
Supplement: Supplementary file 7 [file reference_rows.tex]

M3B & 16--24 & 1--4 & 0/9 \\
Q7B & 12--18 & 4--18 & 7/7 \\
M8B & 25--31 & 0--4 & 0/7 \\
L8B & 15--22 & 17--22 & 6/8 \\
Q14B & 25--31 & 23--29 & 5/7 \\
M14B & 16--21 & 7--13 & 0/6 \\
