# Supplementary material for: Transferring an analysis of human brain organization to language models
Source: arXiv:2611.24626 source file (2026-11-18)
Supplement: Supplementary file 8 [file selector_accuracy_rows.tex]

M3B & MATH-87 & 78.93 & 82.76 & 66.67 & 80.84 & 66.28 \\
 & AIME 2024 & 26.67 & 35.83 & 13.61 & 31.67 & 20.28 \\
 & AIME 2025 & 13.06 & 25.00 & 16.11 & 22.78 & 14.44 \\
\addlinespace[3pt]
Q7B & MATH-87 & 78.16 & 78.93 & 73.56 & 76.25 & 76.63 \\
 & AIME 2024 & 11.94 & 17.50 & 13.61 & 13.06 & 12.22 \\
 & AIME 2025 & 10.00 & 17.50 & 10.56 & 8.06 & 11.39 \\
\addlinespace[3pt]
M8B & MATH-87 & 83.14 & 83.91 & 80.46 & 83.52 & 78.54 \\
 & AIME 2024 & 35.56 & 43.06 & 28.06 & 35.28 & 31.94 \\
 & AIME 2025 & 27.22 & 29.72 & 20.83 & 28.33 & 25.28 \\
\addlinespace[3pt]
L8B & MATH-87 & 41.00 & 47.89 & 41.00 & 41.00 & 44.06 \\
 & AIME 2024 & 5.00 & 3.06 & 1.94 & 1.94 & 3.89 \\
 & AIME 2025 & 0.83 & 1.67 & 1.39 & 1.39 & 1.67 \\
\addlinespace[3pt]
Q14B & MATH-87 & 74.33 & 78.16 & 74.71 & 68.97 & 68.58 \\
 & AIME 2024 & 14.17 & 19.44 & 14.17 & 8.61 & 9.44 \\
 & AIME 2025 & 13.33 & 17.22 & 11.67 & 10.56 & 15.00 \\
\addlinespace[3pt]
M14B & MATH-87 & 86.21 & 89.27 & 86.21 & 87.74 & 89.27 \\
 & AIME 2024 & 48.06 & 47.50 & 42.22 & 37.50 & 47.50 \\
 & AIME 2025 & 31.39 & 35.56 & 28.61 & 27.78 & 35.56 \\
