# Supplementary material for: Transferring an analysis of human brain organization to language models
Source: arXiv:2611.24626 source file (2026-11-18)
Supplement: Supplementary file 9 [file selector_span_rows.tex]

M3B & 16--24 & 0--8 & 12--20 & 8--16 \\
Q7B & 12--18 & 18--24 & 20--26 & 10--16 \\
M8B & 25--31 & 1--7 & 27--33 & 13--19 \\
L8B & 15--22 & 21--28 & 21--28 & 11--18 \\
Q14B & 25--31 & 1--7 & 41--47 & 19--25 \\
M14B & 16--21 & 0--5 & 8--13 & 16--21 \\
