# Supplementary material for: Transferring an analysis of human brain organization to language models
Source: arXiv:2611.24626 source file (2026-11-18)
Supplement: Supplementary file 10 [file threshold_rows.tex]

M3B & 16--24 & 16--24 & 16--24 & 17--24 & 17--24 & 18--24 & 18--21 \\
Q7B & 10--18 & 11--18 & 12--18 & 12--17 & 4--7 & 4--7 & 4--7 \\
M8B & 2--9 & 25--31 & 25--31 & 25--30 & 26--30 & 26--30 & 26--30 \\
L8B & 1--28 & 12--27 & 13--27 & 14--26 & 15--23 & 15--22 & 15--19 \\
Q14B & 25--31 & 25--31 & 25--31 & 25--31 & 25--31 & 25--31 & 25--31 \\
M14B & 17--22 & 17--22 & 16--21 & 16--21 & 16--21 & 16--21 & 16--21 \\
